# Supplementary material for: Optical magnons with dominant bond-directional exchange interactions in a honeycomb lattice iridate $\alpha$-Li$_{2}$IrO$_{3}$
Source: arXiv:2101.03471 source file (2021-01-10)
Supplement: Supplementary file 1 [file SM_Chun_a-Li2IrO3.pdf]

Supplemental Material for

**Optical magnons with dominant bond-directional exchanges in a honeycomb  
lattice iridate  $\alpha$ -Li<sub>2</sub>IrO<sub>3</sub>**

Sae Hwan Chun,<sup>1,2,3,\*</sup> P. Peter Stavropoulos,<sup>2</sup> Hae-Young Kee,<sup>2,4</sup> M. Moretti Sala,<sup>5,6</sup> Jungho Kim,<sup>7</sup> Jong-Woo Kim,<sup>7</sup> B. J. Kim,<sup>8,9</sup> J. F. Mitchell,<sup>1</sup> and Young-June Kim<sup>2</sup>

<sup>1</sup>*Materials Science Division, Argonne National Laboratory, Argonne, Illinois 60439, USA*

<sup>2</sup>*Department of Physics, University of Toronto, 60 St. George Street, Toronto, Ontario M5S 1A7, Canada*

<sup>3</sup>*Pohang Accelerator Laboratory, Pohang, Gyeongbuk 37673, Republic of Korea*

<sup>4</sup>*Canadian Institute for Advanced Research, Toronto, Ontario, M5G 1Z8, Canada*

<sup>5</sup>*ESRF, The European Synchrotron, 71 Avenue des Martyrs, F-38000 Grenoble, France*

<sup>6</sup>*Dipartimento di Fisica, Politecnico di Milano, Piazza Leonardo da Vinci 32, I-20133 Milano, Italy*

<sup>7</sup>*Advanced Photon Source, Argonne National Laboratory, Argonne, Illinois 60439, USA*

<sup>8</sup>*Department of Physics, Pohang University of Science and Technology, Pohang, Gyeongbuk 37673, Republic of Korea*

<sup>9</sup>*Center for Artificial Low Dimensional Electronic Systems, Institute for Basic Science (IBS), 77 Cheongam-Ro, Pohang, Gyeongbuk 37673, Republic of Korea*

\*E-mail: [pokchun81@gmail.com](mailto:pokchun81@gmail.com)

### 1. Ambiguity of acoustic magnon mode in the RIXS spectrum

We attempt to fit the RIXS spectrum with three Gaussian peaks in order to separate elastic background ( $E = 0$  peak), acoustic magnon, and optical magnon modes. Top and bottom panels of Fig. S1 show the fitting results taking into account different contributions from the  $E = 0$  peak (black), acoustic magnon mode (orange), and optical magnon modes (pink). It is noted that distinct spectrum profiles of the acoustic mode account for the data equally well. This insensitivity to the fitting results makes it hard to unambiguously identify the acoustic mode from the RIXS spectrum.

Instead of the acoustic mode, we turn our attention to the optical modes. We first look into RIXS spectrum at  $\mathbf{q}_{\text{mag}}$ . Since the RIXS intensity in the elastic peak at this  $\mathbf{q}$  should have contributions from both  $E = 0$  peak and a gapless (or small gap much smaller than the resolution) acoustic magnon, subtraction of the  $E = 0$  peak from the raw spectrum leaves the spectrum from the optical modes (See Fig. S2). This inelastic spectrum can be compared with spectra at the other  $\mathbf{q}$  values. It is evident in the raw data (squares), i.e. without subtraction of the  $E = 0$  peak, that the peaks in the latter are located at lower energy than the former. The damped harmonic oscillator model employed in this work gives the best fit when the elastic background is subtracted at all  $\mathbf{q}$ . The  $E = 0$  peak at  $\mathbf{q} \neq \mathbf{q}_{\text{mag}}$  is rather insignificant in the raw data, and thereby the inelastic spectral weight in the energy range 20-25 meV depends only weakly on the subtraction procedure.

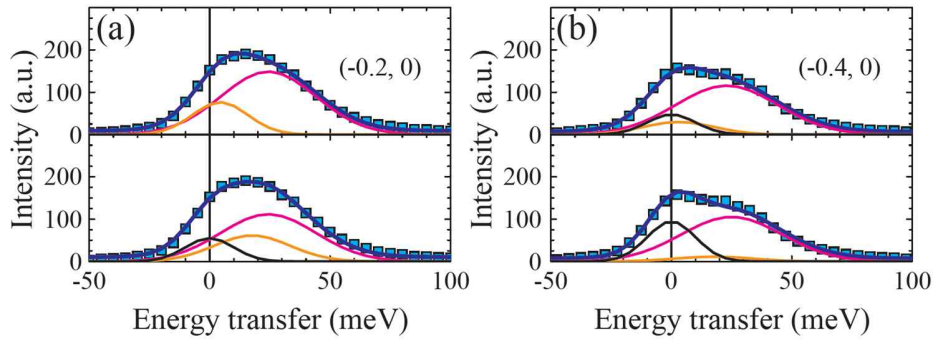

**Figure S1** | Fitting results (blue) of the raw RIXS spectrum (square symbol) at  $\mathbf{q} =$  (a)  $(-0.2, 0)$  and (b)  $(-0.4, 0)$ . Top and bottom panels at each  $\mathbf{q}$  consider different contributions from elastic background (black), acoustic magnon mode (orange), and optical magnon modes (pink).

## 2. Optical magnons observed in multiple Brillouin zones

Momentum dependence of spectral weights associated with optical magnon bands are expected to show a periodic characteristic for multiple Brillouin zones. We measured the RIXS spectra not only in a Brillouin zone centered at  $\mathbf{Q} = (0, 0)$ , but also in other Brillouin zones. The spectra are analyzed by the damped harmonic oscillator (DHO) model:

$$S(\mathbf{q}, \omega) = \frac{A(\mathbf{q})}{1 - \exp(-\hbar\omega/k_B T)} \left[ \frac{\gamma_q}{(\hbar\omega - \hbar\omega_q)^2 + \gamma_q^2} - \frac{\gamma_q}{(\hbar\omega + \hbar\omega_q)^2 + \gamma_q^2} \right],$$

where  $\omega_q$  is the peak position,  $\gamma_q$  is the peak width,  $A(\mathbf{q})$  is the overall amplitude,  $\hbar$  is Planck's constant, and  $k_B$  is Boltzmann's constant. The elastic background ( $E = 0$  peak) is fitted on the energy gain side (energy transfer  $< 0$ ) with the instrumental resolution function (energy resolution  $\sim 24$  meV). The spectrum subtracted by the elastic intensity is fitted with the DHO model. Figure S1 shows the raw spectra along the  $h$  direction at several Brillouin zones centered at  $\mathbf{Q} = (-2, -2)$ ,  $(3, 3)$ , and  $(2, 0)$ . It is noted for all of the Brillouin zones that the spectrum arising from the optical magnon modes (pink curve) shows the dispersion that reaches the highest energy  $\sim 25$  meV at  $\mathbf{q}_{\text{mag}} = (\pm 0.32, 0)$  and then monotonically decreases down to  $\sim 20$  meV moving away from  $\mathbf{q}_{\text{mag}}$ .

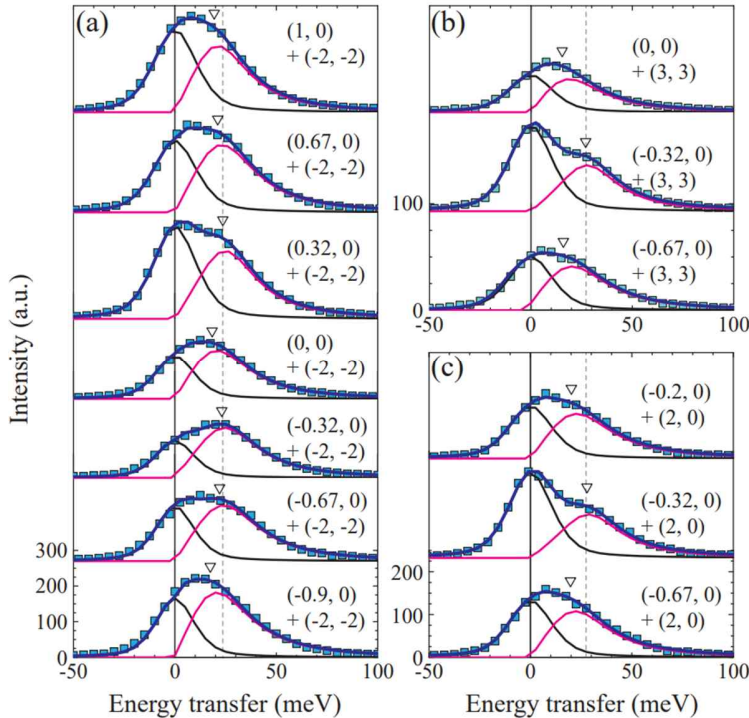

**Figure S2** | RIXS spectra at 4 K along  $(h, 0)$  in different Brillouin zones centered at (a)  $(-2, -2)$ , (b)  $(3, 3)$ , and (c)  $(2, 0)$ . Each spectrum is vertically shifted for clarity. Raw spectrum is depicted by square symbol. Black and pink curves correspond to the  $E = 0$  peak and inelastic peak fitted with a damped harmonic oscillator (DHO) model, respectively. Their sum (blue curve) is overlaid on the raw data. Triangle denotes the peak energy obtained by the DHO fitting. Dashed line denotes the peak energy at  $\mathbf{q}_{\text{mag}}$  for a guide to the eye.

### 3. Linear spin-wave theory calculation for different exchange parameter sets

This work employs a magnetic Hamiltonian,

$$H = \sum_{\langle ij \rangle_\gamma} [K S_i^\gamma S_j^\gamma + \Gamma (S_i^\alpha S_j^\beta + S_i^\beta S_j^\alpha) + \Gamma' (S_i^\alpha S_j^\gamma + S_i^\gamma S_j^\alpha + S_i^\beta S_j^\gamma + S_i^\gamma S_j^\beta) + J \mathbf{S}_i \cdot \mathbf{S}_j],$$

where  $\langle ij \rangle_\gamma$  denotes a nearest-neighbor  $\gamma$ -bond ( $\gamma \neq \alpha \neq \beta \in (x, y, z)$ );  $K$  is the Kitaev interaction,  $\Gamma$  is symmetric off-diagonal exchange interaction,  $\Gamma'$  is the additional exchange arising from trigonal distortion of the octahedron, and  $J$  is the usual isotropic Heisenberg exchange interaction. It is noted that the counter-rotating spiral order in  $\alpha$ -Li<sub>2</sub>IrO<sub>3</sub> cannot be formed only by the  $K$  and  $J$  terms [1], but by the combination of  $K$ ,  $\Gamma$ ,  $\Gamma'$ , and  $J$  terms: the magnetic order is stabilized mainly by ferromagnetic  $K$  and antiferromagnetic  $\Gamma$ , while both  $\Gamma'$  and  $J$  play minor roles [2, 3]. This magnetic ground state constrains the ranges of the magnetic exchange parameters for linear spin-wave theory calculation.

Our RIXS data are not sufficiently detailed enough to identify the exchange parameters by a fitting process. Instead, we explore the ranges of the parameters that can reproduce main features observed in the RIXS spectra: 1) momentum dependence of the inelastic spectral weight reaching the highest energy  $\sim 25$  meV at  $\mathbf{q}_{\text{mag}}$  and monotonically decreasing down to  $\sim 20$  meV at  $\mathbf{q} = (0, 0)$  and the Brillouin zone boundary along the  $h$  direction; 2) a gapless (or small gap much smaller than the energy resolution) acoustic magnon at  $\mathbf{q}_{\text{mag}}$  whose intensity is drastically reduced moving away from  $\mathbf{q}_{\text{mag}}$ ; 3) substantial spectral weight of optical magnon modes compared with that of the acoustic mode.

Figure S3 shows examples of magnon dispersions along the  $h$  direction ( $0 \leq h \leq 1$ ) calculated by the linear spin-wave theory for different sets of parameters with an approximation,  $\mathbf{q}_{\text{mag}} = (1/3, 0)$ . It is found that the optical magnon modes gain more spectral weight for  $|K| > |\Gamma|$  as in the RIXS data and their energy scale is predominantly determined by  $|K|$ . The spin wave dispersion changes slightly depending on the ratio of  $\Gamma'$  and  $J$ . We tune the parameters that can account for our observation satisfactorily and select one putative parameter set,  $K = -25$  meV,  $\Gamma = 17.4$  meV,  $\Gamma' = 3.2$  meV, and  $J = 4.4$  meV. Figure S4 presents the magnon dispersions that are symmetrized for  $\pm h$  and convoluted with instrumental resolution functions, e.g. Gaussian functions with the

momentum width  $\Delta q \sim 0.1$  r.l.u. and the energy width  $\Delta E \sim 24$  meV. This simulation convinces that one can observe momentum dependence of inelastic feature around the energy scale of the Kitaev interaction, which is formed by the combination of several optical magnon modes with scattering intensities dependent on the momentum. Therefore,  $K$  could be identified even without making a sharp, quantitative statement on the other exchange interactions.

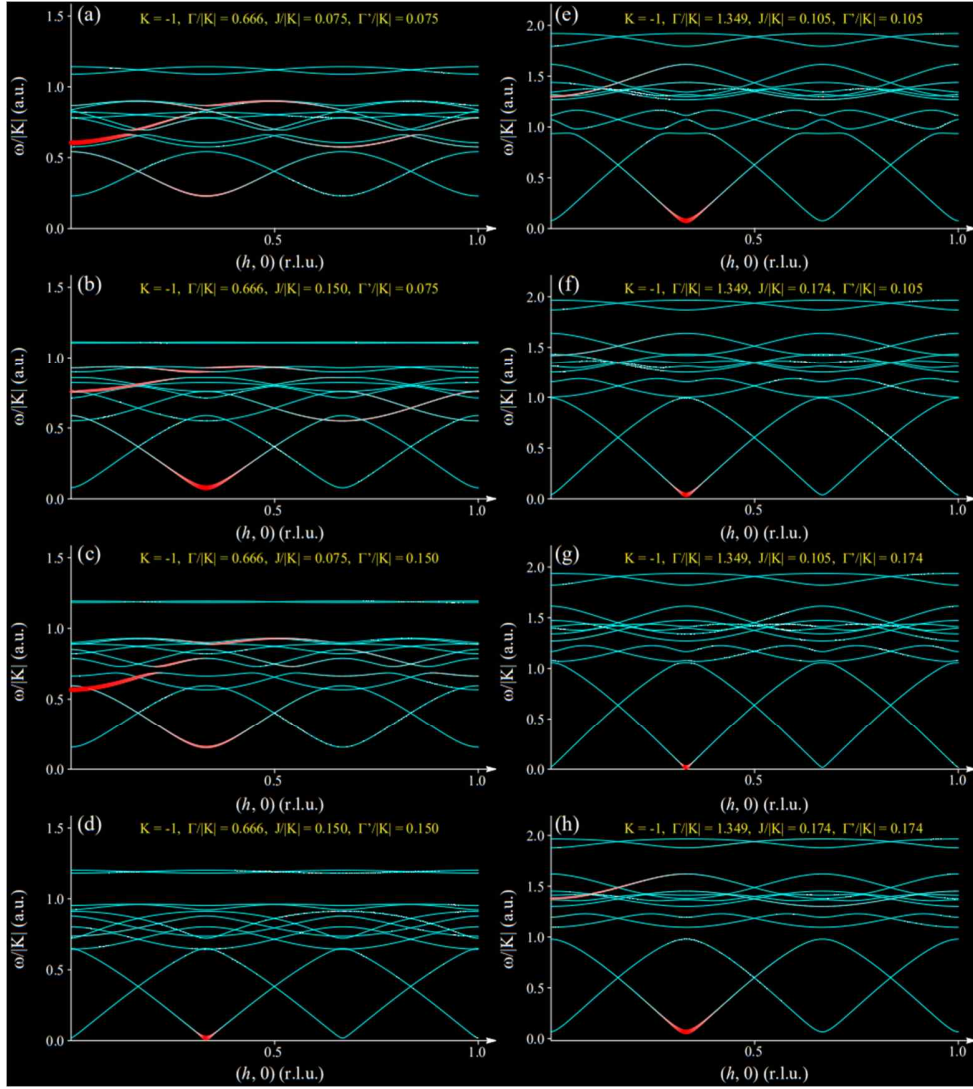

**Figure S3** | Calculated magnon dispersions by the linear spin-wave theory for various sets of the exchange parameters. The exchange parameters and magnon energies are scaled by the Kitaev exchange interaction,  $|K|$ . (a)  $(K, \Gamma, \Gamma', J) = (-1, 0.666, 0.075, 0.075)$ , (b)  $(-1, 0.666, 0.15, 0.075)$ , (c)  $(-1, 0.666, 0.075, 0.15)$ , (d)  $(-1, 0.666, 0.15, 0.15)$ , (e)  $(-1, 1.349, 0.105, 0.105)$ , (f)  $(-1, 1.349,$

0.174, 0.105), (g) (-1, 1.349, 0.105, 0.174), and (h) (-1, 1.349, 0.174, 0.174). The magnon bands are denoted with cyan curves and their intensities are plotted in a pseudo-color scale.

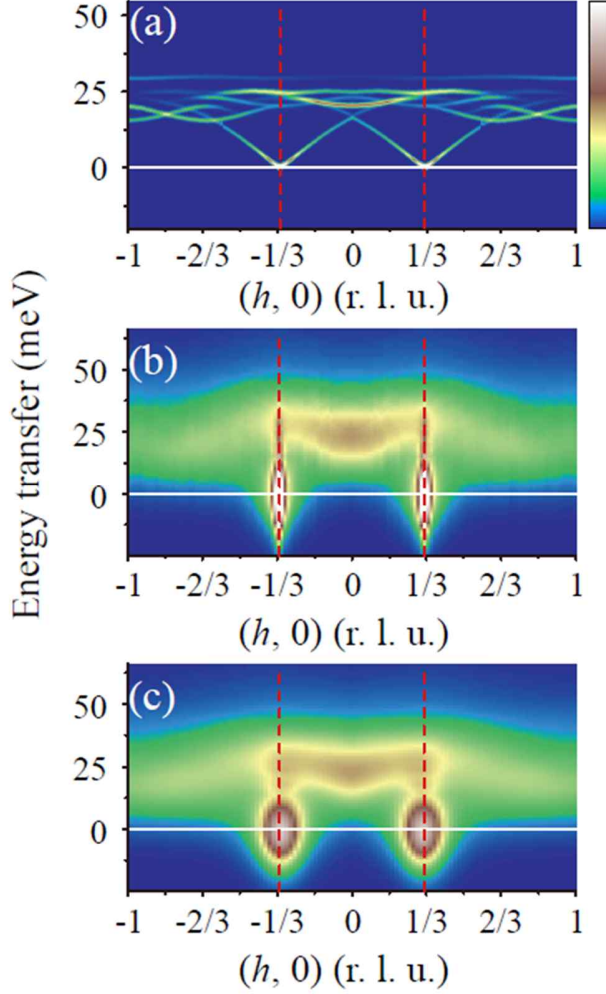

**Figure S4** | A simulation result of magnon dispersions convoluted with instrumental resolution functions. (a) The spin-wave theory calculation result for  $K = -25$  meV,  $\Gamma = 17.4$  meV,  $\Gamma' = 3.2$  meV, and  $J = 4.4$  meV. These magnon spectra are convoluted with the energy resolution  $\Delta E \sim 24$  meV (b) and then followed by another convolution process with the momentum resolution  $\Delta q \sim 0.1$  r.l.u. (c).

## References

- [S1] S. C. Williams, R. D. Johnson, F. Freund, S. Choi, A. Jesche, I. Kimchi, S. Manni, A. Bombardi, P. Manuel, P. Gegenwart, and R. Coldea, *Phys. Rev. B* **93**, 195158 (2016).
- [S2] J. G. Rau, E. K.-H. Lee, and H.-Y. Kee, *Phys. Rev. Lett.* **112**, 077204 (2014).
- [S3] J. G. Rau and H.-Y. Kee, arXiv:1408.4811 (2014).
